# Supplementary material for: Fooling LIME and SHAP: Adversarial Attacks on Post hoc Explanation Methods
Source: arXiv:1911.02508 source file (2020-02-03)
Supplement: Supplementary file 1 [file appendix.tex]

\clearpage

% \twocolumn[{\centering{\Large Appendix}}]
\onecolumn
% \section*{Appendix}
\appendix
\setcounter{secnumdepth}{1} 
\section*{Appendices}
% \renewcommand{\thesubsection}{\Alph{subsection}}

% \section{Details of the Algorithms}

\begin{table}[h]
\begin{center}
\begin{tabular}{  c p{135mm} } 
 \toprule
\bf Symbol & \bf Description \\
\midrule
\addlinespace
 $x_i$ & Observed attributes of a data point $i$ \\ \addlinespace
 $y_i$ & ground truth class label of a data point $i$\\
 \addlinespace
 $\mathcal{X}$ & Set of all the observed attributes of input data points i.e., $\mathcal{X} = \{x_1, x_2, \cdots x_N\}$\\ \addlinespace
  $\bm{y}$ & Set of all the ground truth class labels of input data points  i.e., $\bm{y} = \{y_1, y_2, \cdots y_N\}$\\ \addlinespace
 $\mathcal{D}$ & Set of input data points $\mathcal{D} = (\mathcal{X},\bm{y}) = \{(x_1, y_1), (x_2, y_2) \cdots (x_N, y_N)\}$\\ \addlinespace
  $\mathcal{C}$ & Set of class labels in $\mathcal{D}$ i.e., $\forall i$, $y_i \in \mathcal{C}$\\\addlinespace
% $\boldmath{x}_i$ & Datapoint $i$\\ \\
$\mathcal{X}_{dist}$ & Distribution from which $\mathcal{X}$ is sampled \\ \addlinespace
$\mathcal{D}_{dist}$ & Distribution from which $\mathcal{D}$ is sampled \\ \addlinespace
 $f$ & Black box model which maps a data point %\\
 %$\mathcal{B}(\boldmath{x}_i)$ & Prediction of black box model on datapoint $\boldmath{x}_i$,  \\
%  & 
 to a class label i.e., $f(x_i) \in \mathcal{C}$\\
 \addlinespace
 $g$ & Interpretable model that serves as an explanation of the black box model $f$ generated by posthoc explanation techniques \\ \addlinespace
 $\psi$ & Unbiased classification function \\ \addlinespace
 $e$ & Adversarial classifier \\ \addlinespace
 $\mathcal{X}_p$ & Set of perturbed data points generated from $\mathcal{X}$ \\ \addlinespace
 \bottomrule
%  \vspace{0.01in}
\end{tabular}
% \vspace{0.2in}
\end{center}
\caption{Description of Notation}
\end{table}

\begin{table*}[h]
\begin{tabular}{lcccccccc}
\toprule
\multicolumn{8}{l}{\bf COMPAS LIME Adversarial Classifier}                                                                                                                                     \\ 
% Number of Uncorrelated Columns & 
 & 
\multicolumn{1}{c}{Baseline classifier $f$}                                                       & \multicolumn{3}{c}{Attack 1 feature}                                                       & \multicolumn{3}{c}{Attack 2 features}    \\ 
\cmidrule(lr){2-2}
\cmidrule(lr){3-5}
\cmidrule(lr){6-8}

% \addlinespace
Importance Ranking     & 1                                  & 1                     & 2                     & 3      & 1      & 2      & 3      \\ \midrule

% Male                           & 0      & 0                 & 1 1\%                & 20 2\% & 0    &0    & 10 4\%\\ %

African-American            
                              & 100 & 0   & 9    & 11 & 0  & 0 & 11 \\ %
\addlinespace
Unrelated Feature 1      
                             & 0      & 100         & 0      & 0     & 49 & 51     & 0    \\
% \addlinespace
Unrelated Feature 2       
                             & 0        & 0    & 9  & 10  & 50    & 49    & 0    \\
 \addlinespace
Other Features &  0 & 0 & 82  & 79 & 0 & 0 & 89 \\ \midrule
Accuracy & 56 & & 56 & & & 56 &   \\                             \bottomrule
\end{tabular}
\centering

\vspace{3mm}

\begin{tabular}{lcccccccc}
\toprule
\multicolumn{8}{l}{\bf COMPAS SHAP Adversarial Classifier}                                                                                                                                     \\ 

 & 
\multicolumn{1}{c}{Baseline classifier $f$}                                                       & \multicolumn{3}{c}{Attack 1 feature}                                                       & \multicolumn{3}{c}{Attack 2 features}    \\ 
\cmidrule(lr){2-2}
\cmidrule(lr){3-5}
\cmidrule(lr){6-8}
Importance Ranking     & 1                                  & 1                     & 2                     & 3      & 1      & 2      & 3      \\ \midrule

\addlinespace

African-American    & 100   & 16      & 82      & 1  & 34   & 31 & 33   \\ %

\addlinespace
Unrelated Feature 1  & 0      & 84     & 12   & 1   & 35  & 31   & 19  \\
% \addlinespace
Unrelated Feature 2 
 & 0        & 0    & 0    & 13    & 32  & 31  & 18 \\ 
 
 Other Features &  0 & 0 & 6  & 55 & 0 & 5 & 20 \\ \midrule

 Accuracy  & 56 & & 53  & & & 55  &   \\                   
 \bottomrule
\end{tabular}
\centering
\caption{The percentage occurrence of the top features in $e$ with the perfectly unfair $f$ (if African-American predict high likely to recidivate) on COMPAS LIME and SHAP adversarial explanations.  ``Attack 1 feature'' and ``Attack 2 features'' can be read as two different scenarios: the former where one feature is used in $\psi$ and the latter where two features are used in $\psi$. The baseline is the explanation on $f$.  The percentages are the mean rates of occurrences on a 10\% test set over three different runs (including re splitting into a different train-test set).   We see that whether the individual is African American is the most important feature in both LIME and SHAP on $f$.  Using $e$, we are able to exclude all of the explanations of this feature in LIME and most of the explanations in SHAP in the top feature positions.
% \sameer{total instead of average}
% \sameer{try to fit these side by side (first column is the same)}
}
\label{table:COMPAS}
\end{table*}

% \begin{table*}[h]
% \begin{tabular}{  lc}
% \toprule
% \multicolumn{8}{l}{\bf COMPAS LIME Adversarial Classifier}                                                                                                                                     \\ 
% % Number of Uncorrelated Columns & 
%  & 
% \multicolumn{1}{c}{Baseline}                                                       & \multicolumn{3}{c}{Attack 1 feature}                                                       & \multicolumn{3}{c}{Attack 2 features}    \\ 
% \cmidrule(lr){2-2}
% \cmidrule(lr){3-5}
% \cmidrule(lr){6-8}

% % \addlinespace
% Importance Ranking     & 1                                  & 1                     & 2                     & 3      & 1      & 2      & 3      \\ \midrule

% % Male                           & 0      & 0                 & 1 1\%                & 20 2\% & 0    &0    & 10 4\%\\ %

% African-American               & 100 0 & 0 0    & 10 0    & 10 0 & 0 0   & 0 0 & 10 0  \\ %
%                               & 100    & 0       & 9 1\%    & 11 1\% & 0      & 0    & 11    \\ %
% \addlinespace
% Unrelated Feature 1          & 0 0   & 100 0      & 0 0   & 0 0  & 49 0 & 51 0  & 0 0 \\ %
%                              & 0      & 100         & 0      & 0     & 49 1\% & 51     & 0    \\
% \addlinespace
% Unrelated Feature 2          & 0 0     & 0 0 & 9 0 & 10 0  & 51 0 & 49 1 & 10 1\\
%                              & 0        & 0    & 9 1\% & 10 1\%  & 50    & 49    & 0    \\ \midrule
% Accuracy & 41 1\%& & 41 1\% & & &41 1\% &   \\                             \bottomrule
% \end{tabular}
\centering

\vspace{3mm}
\begin{table*}[h]
\begin{tabular}{lcccccccc}
\toprule
\multicolumn{8}{l}{\bf Communities and Crime LIME Adversarial Classifier}                                                                                                                                     \\ 
% Number of Uncorrelated Columns & 
 & 
\multicolumn{1}{c}{Baseline classifier $f$}                                                       & \multicolumn{3}{c}{Attack 1 feature}                                                       & \multicolumn{3}{c}{Attack 2 features}    \\ 
\cmidrule(lr){2-2}
\cmidrule(lr){3-5}
\cmidrule(lr){6-8}
Importance Ranking     & 1                                  & 1 & 2       & 3      & 1      & 2      & 3      \\ \midrule

Race \% White     & 100   & 0        & 1        & 1  & 0     & 0    & 2  \\ %

\addlinespace
Unrelated Feature 1  & 0      & 100        & 0      & 0    & 48  & 52   & 0   \\
% \addlinespace
Unrelated Feature 2  & 0        & 0    & 3    & 3  & 52  & 48  & 0    \\ 
 
  \addlinespace
Other Features  &  0 & 0 & 96  & 96 & 0 & 0 & 98 \\ \midrule

 Accuracy   & 73  & & 73  & & &73  &   \\                   
 \bottomrule
\end{tabular}
\centering

\vspace{3mm}

\begin{tabular}{lcccccccc}
\toprule
\multicolumn{8}{l}{\bf Communities and Crime SHAP Adversarial Classifier}                                                                                                                                     \\ 
% Number of Uncorrelated Columns & 
 & 
\multicolumn{1}{c}{Baseline classifier $f$}                                                       & \multicolumn{3}{c}{Attack 1 feature}                                                       & \multicolumn{3}{c}{Attack 2 features}    \\ 
\cmidrule(lr){2-2}
\cmidrule(lr){3-5}
\cmidrule(lr){6-8}
Importance Ranking     & 1                                  & 1                     & 2                     & 3      & 1      & 2      & 3      \\ \midrule

Race \% White     & 100   & 0        & 78   & 3  & 26 & 26 & 40  \\ %

\addlinespace
Unrelated Feature 1  & 0      & 100        & 0      & 0    & 36  & 25   & 7 \\
% \addlinespace
Unrelated Feature 2  & 0        & 0    & 0    & 3  & 35  & 30  & 6  \\ 

\addlinespace
Other Features &  0 & 0 & 16  & 86 & 0 & 16 & 44 \\

\midrule

 Accuracy    & 73 & & 70  & & &72  &   \\                   
 \bottomrule
\end{tabular}
\centering
\caption{The percentage occurrence of the top features in $e$ with the perfectly unfair $f$ (if race \% white $>$ median race \% white predict nonviolent community) on Communities and Crime.  Using the $e$, we are able to exclude all of the explanations of this feature in LIME and many of the SHAP explanations, consistent with our results on COMPAS.}
\label{table:CC}
\end{table*}

\begin{table}[h]
\begin{tabular}{lcccc}
\toprule
\multicolumn{5}{l}{\bf German Credit LIME Adversarial Classifier}                                                                                                                                     \\ 
% Number of Uncorrelated Columns & 
 & 
\multicolumn{1}{c}{Baseline classifier $f$}                                                       & \multicolumn{3}{c}{With Attack}                                                \\ 
\cmidrule(lr){2-2}
\cmidrule(lr){3-5}

Importance Ranking     & 1                                  & 1                     & 2                     & 3      \\ \midrule

\addlinespace

Gender    & 100   & 0      & 4      & 4   \\ %

\addlinespace
Loan Rate \% Income  & 0      & 91     & 0   & 0  \\

 Other Features  &  0 & 9 & 96  & 96 \\ \midrule

 Accuracy  & 64 & & 64  &    \\                   
 \bottomrule
\end{tabular}
\centering

\vspace{3mm}

\begin{tabular}{lcccc}
\toprule
\multicolumn{5}{l}{\bf German Credit SHAP Adversarial Classifier}                                                                                                                                     \\ 
% Number of Uncorrelated Columns & 
 & 
\multicolumn{1}{c}{Baseline classifier $f$}                                                       & \multicolumn{3}{c}{With Attack}                                                \\ 
\cmidrule(lr){2-2}
\cmidrule(lr){3-5}

Importance Ranking     & 1                                  & 1                     & 2                     & 3      \\ \midrule

\addlinespace

Gender    & 100   & 0      & 5      & 1   \\ %

\addlinespace
Loan Rate \% Income  & 0      & 85     & 0   & 0  \\

 Other Features &  0 & 0 & 72  & 65 \\ \midrule

 Accuracy  & 64 & & 64  &    \\                   
 \bottomrule
\end{tabular}
\centering
\caption{The percentage occurrence of the top features in $e$ with the perfectly unfair $f$ (if Gender is male predict will repay loan) on COMPAS LIME and SHAP explanations.  We use loan rate as a percentage of income as $\psi$ and predict false if the value is above its mean.  In both the LIME and SHAP case, we are able to exclude gender from the majority of the explanations.  When the explanation is included, it appears at the same frequency as other features.}
\end{table}

% \clearpage
% \section{Detailed Results of the LIME/SHAP Hyperparameters}
\label{sec:hyperparams}

\begin{figure}[h]
    \centering
    \includegraphics[width=.5\columnwidth,clip,trim=20 0 0 0]{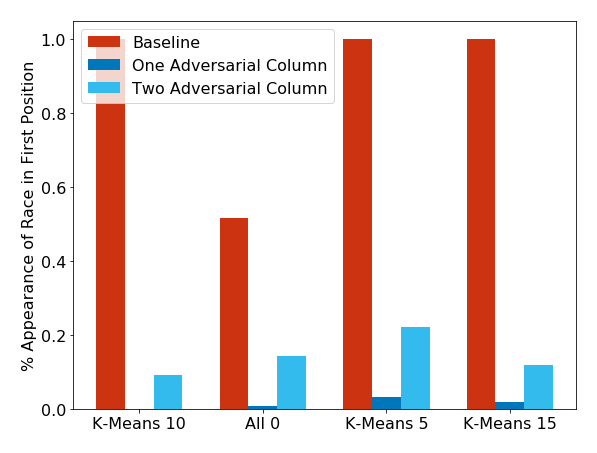}
    \caption{SHAP attack effectiveness across different background distributions: K-means 10 is the distribution assumed in training. We also test on K-means 5, K-means 15, and all 0. These represent different suggestions in the SHAP software package for representing a large dataset.}
    \label{fig:shap_sensitivity}
\end{figure}

\begin{figure}[H]
    \centering
    \includegraphics[width=.5\columnwidth]{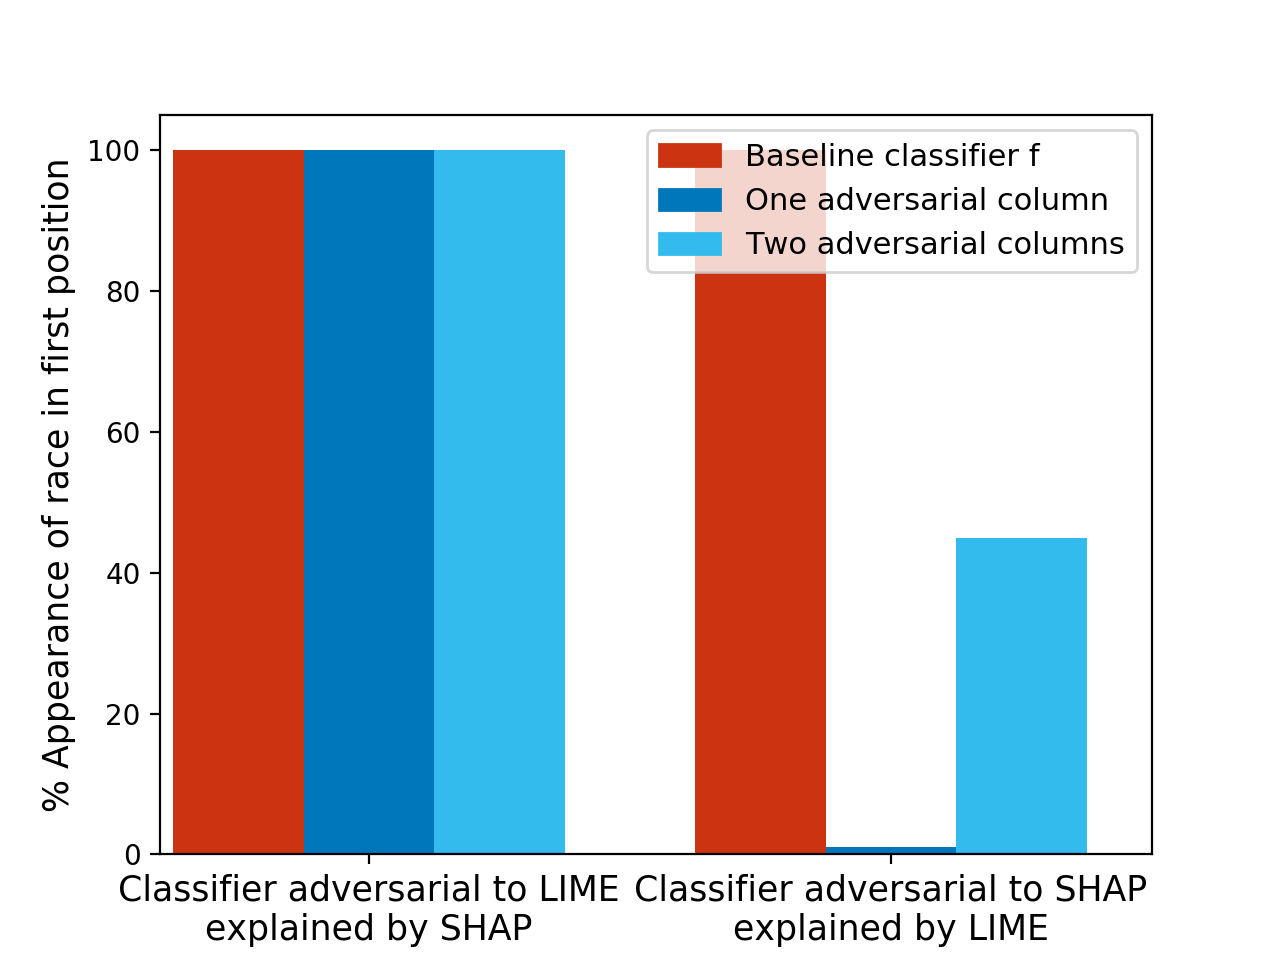}
    \caption{The effectiveness of explaining classifiers adversarial to SHAP with LIME and classifiers adversarial to LIME with SHAP. We see that classifiers adversarial to LIME are not effective at hiding bias from SHAP explanations, and classifiers adversarial to SHAP are moderately effective at hiding biases from LIME explanations.}
    \label{fig:shaponlimelimeonshap}
\end{figure}

% \begin{algorithm}[h]
% \caption{Building OOD Sample Detection Classifier}
% \label{alg:ood}
% \begin{algorithmic}[1]
% \State \textbf{Input:} Input data $\mathcal{X}$; $\texttt{perturb}()$;  
% \State \textbf{Output:} OOD Sample Detection Classifier
% % \\
%  \State $\mathcal{X}_{p}$ = \{\} \Comment{Set of perturbed data points}\\
%  \For{$x \in \mathcal{X}$}\\
%  \hspace{2em}$x_p = \texttt{perturb}(x)$\\
%  \hspace{2em}$\mathcal{X}_p = \mathcal{X}_p \cup x_p$
%  \EndFor\\
%  \State \For{$x \in \mathcal{X}$}\Comment{Input data points are not OOD}\\
%  \hspace{2em} assign label $\texttt{False}$ 
%  \EndFor
%  \State \For{$x_p \in \mathcal{X}_p$}\Comment{Check if a perturbed point is OOD}
%  \hspace{2em} Assign label $\texttt{True}$ 
%  \If {$\exists x \in \mathcal{X}, x_p \approx x$} assign label $\texttt{False}$
%  \Else {} assign label $\texttt{True}$
%  \EndIf 
%  \EndFor\\
%  \State
%  Train a classifier $\texttt{is\_OOD}$ on $\mathcal{X} \cup \mathcal{X}_p$ and their corresponding labels (assigned above).  \\ \\

%  \Return $\texttt{is\_OOD}$

% \end{algorithmic}
% \end{algorithm}

% \begin{algorithm}[h]
% \caption{Adversarial Classifier $e$}
%  \label{alg:adv}
% \begin{algorithmic}[1]
% \State \textbf{Input:} Biased Base classifier $f$; Unbiased classifier $\psi$; \\ Sample data point $x$; $\texttt{is\_OOD}()$;  
% \State \textbf{Output:} Prediction of adversarial classifier $e$ on input data point $x$\\
% \If {\textbf{not}   $\texttt{is\_OOD}(x)$} $e_x = f(x)$
% \Else {} $e_x = \psi(x)$
% \EndIf 
% %\EndFor
% \\
% \\
% \Return $e_x$
% \end{algorithmic}
% \end{algorithm}
